# Supplementary material for: Construction of a series of new $\nu=2/5$ fractional quantum Hall wave functions by conformal field theory
Source: arXiv:2006.15814 source file (2020-09-16)
Supplement: Supplementary file 1 [file supplement_7.2.pdf]

# Supplemental Material for "Construction of a series of topologically distinct $\nu = 2/5$ fractional quantum Hall wave functions by conformal field theory"

Li Chen[1] and Kun Yang[2]

[1]*College of Physics and Electronic Science, Hubei Normal University, Huangshi 435002, China*

[2]*National High Magnetic Field Laboratory and Department of Physics, Florida State University, Tallahassee, FL 32306, USA*

(Dated: September 5, 2020)

## I. THE DENSEST ZERO ENERGY GROUND STATES OF $P_4^{(6)}$ AND $P_4^{(8)}$ ON DISK.

We have chosen a linear combination of $P_4^{(6)}$ and $P_4^{(8)}$ on disk with positive coefficients as the parent Hamiltonian and diagonalized it for up to 10 particles. Since both $P_4^{(6)}$ and $P_4^{(8)}$ are positive-semidefinite projectors, zero energy ground states of the total parent Hamiltonian are zero energy ground states of individual projector. For 4, 5, 6, 8, and 10 particles, there is a unique densest zero energy ground state. Here we list its second-quantized expression without normalization factor. The expression for 10 particles is too long to be shown here. The hereditary nature of zero energy ground states introduced in Sec. VI of the main paper is clearly seen from expressions below.

For 4 particles, the unique densest zero energy ground state is

$$\propto \left(c_0^\dagger c_1^\dagger c_2^\dagger c_6^\dagger - \sqrt{2} c_0^\dagger c_1^\dagger c_3^\dagger c_5^\dagger + \sqrt{5} c_0^\dagger c_2^\dagger c_3^\dagger c_4^\dagger\right) |0\rangle . \tag{1.1}$$

For 5 particles, the unique densest zero energy ground state is

$$\propto \left(c_0^\dagger c_1^\dagger c_2^\dagger c_6^\dagger c_7^\dagger - \sqrt{2} c_0^\dagger c_1^\dagger c_3^\dagger c_5^\dagger c_7^\dagger + \sqrt{5} c_0^\dagger c_2^\dagger c_3^\dagger c_4^\dagger c_7^\dagger - \sqrt{7} c_0^\dagger c_2^\dagger c_3^\dagger c_5^\dagger c_6^\dagger + \sqrt{14} c_0^\dagger c_1^\dagger c_4^\dagger c_5^\dagger c_6^\dagger\right) |0\rangle . \tag{1.2}$$

For 6 particles, the unique densest zero energy ground state is

$$\begin{aligned} \propto \big(& c_0^\dagger c_1^\dagger c_2^\dagger c_6^\dagger c_7^\dagger c_9^\dagger - \sqrt{2} c_0^\dagger c_1^\dagger c_3^\dagger c_5^\dagger c_7^\dagger c_9^\dagger + \sqrt{5} c_0^\dagger c_2^\dagger c_3^\dagger c_4^\dagger c_7^\dagger c_9^\dagger - \sqrt{7} c_0^\dagger c_2^\dagger c_3^\dagger c_5^\dagger c_6^\dagger c_9^\dagger + \sqrt{14} c_0^\dagger c_1^\dagger c_4^\dagger c_5^\dagger c_6^\dagger c_9^\dagger - \sqrt{3} c_0^\dagger c_1^\dagger c_3^\dagger c_6^\dagger c_7^\dagger c_8^\dagger \\ &+ 4 c_0^\dagger c_2^\dagger c_3^\dagger c_5^\dagger c_7^\dagger c_8^\dagger - 7\sqrt{5} c_1^\dagger c_2^\dagger c_3^\dagger c_4^\dagger c_7^\dagger c_8^\dagger + \sqrt{2} c_0^\dagger c_1^\dagger c_4^\dagger c_5^\dagger c_7^\dagger c_8^\dagger - 4\sqrt{7} c_0^\dagger c_2^\dagger c_4^\dagger c_5^\dagger c_6^\dagger c_8^\dagger + 7\sqrt{7} c_1^\dagger c_2^\dagger c_3^\dagger c_5^\dagger c_6^\dagger c_8^\dagger + 5\sqrt{42} c_0^\dagger c_3^\dagger c_4^\dagger c_5^\dagger c_6^\dagger c_7^\dagger \\ &- 7\sqrt{14} c_1^\dagger c_2^\dagger c_4^\dagger c_5^\dagger c_6^\dagger c_7^\dagger\big) |0\rangle . \end{aligned} \tag{1.3}$$

For 8 particles, the unique densest zero energy ground state is

$$
\begin{aligned}
\propto \big(&c^\dagger_{0}c^\dagger_{1}c^\dagger_{2}c^\dagger_{6}c^\dagger_{7}c^\dagger_{9}c^\dagger_{12}c^\dagger_{13} - 1.41421c^\dagger_{0}c^\dagger_{1}c^\dagger_{3}c^\dagger_{5}c^\dagger_{7}c^\dagger_{9}c^\dagger_{12}c^\dagger_{13} + 2.23607c^\dagger_{0}c^\dagger_{2}c^\dagger_{3}c^\dagger_{4}c^\dagger_{7}c^\dagger_{9}c^\dagger_{12}c^\dagger_{13} - 2.64575c^\dagger_{0}c^\dagger_{2}c^\dagger_{3}c^\dagger_{5}c^\dagger_{6}c^\dagger_{9}c^\dagger_{12}c^\dagger_{13} \\
&+ 3.74166c^\dagger_{0}c^\dagger_{1}c^\dagger_{4}c^\dagger_{5}c^\dagger_{6}c^\dagger_{9}c^\dagger_{12}c^\dagger_{13} - 1.73205c^\dagger_{0}c^\dagger_{1}c^\dagger_{3}c^\dagger_{6}c^\dagger_{7}c^\dagger_{8}c^\dagger_{12}c^\dagger_{13} + 4.0c^\dagger_{0}c^\dagger_{2}c^\dagger_{3}c^\dagger_{5}c^\dagger_{7}c^\dagger_{8}c^\dagger_{12}c^\dagger_{13} - 15.6525c^\dagger_{1}c^\dagger_{2}c^\dagger_{3}c^\dagger_{4}c^\dagger_{7}c^\dagger_{8}c^\dagger_{12}c^\dagger_{13} \\
&+ 1.41421c^\dagger_{0}c^\dagger_{1}c^\dagger_{4}c^\dagger_{5}c^\dagger_{7}c^\dagger_{8}c^\dagger_{12}c^\dagger_{13} - 10.583c^\dagger_{0}c^\dagger_{2}c^\dagger_{4}c^\dagger_{5}c^\dagger_{6}c^\dagger_{8}c^\dagger_{12}c^\dagger_{13} + 18.5203c^\dagger_{1}c^\dagger_{2}c^\dagger_{3}c^\dagger_{5}c^\dagger_{6}c^\dagger_{8}c^\dagger_{12}c^\dagger_{13} + 32.4037c^\dagger_{0}c^\dagger_{3}c^\dagger_{4}c^\dagger_{5}c^\dagger_{6}c^\dagger_{7}c^\dagger_{12}c^\dagger_{13} \\
&- 26.1916c^\dagger_{1}c^\dagger_{2}c^\dagger_{4}c^\dagger_{5}c^\dagger_{6}c^\dagger_{7}c^\dagger_{12}c^\dagger_{13} - 0.912871c^\dagger_{0}c^\dagger_{1}c^\dagger_{2}c^\dagger_{6}c^\dagger_{7}c^\dagger_{10}c^\dagger_{11}c^\dagger_{13} - 3.26599c^\dagger_{0}c^\dagger_{1}c^\dagger_{2}c^\dagger_{6}c^\dagger_{8}c^\dagger_{9}c^\dagger_{11}c^\dagger_{13} + 22.7969c^\dagger_{0}c^\dagger_{1}c^\dagger_{2}c^\dagger_{7}c^\dagger_{8}c^\dagger_{9}c^\dagger_{10}c^\dagger_{13} \\
&+ 1.29099c^\dagger_{0}c^\dagger_{1}c^\dagger_{3}c^\dagger_{5}c^\dagger_{7}c^\dagger_{10}c^\dagger_{11}c^\dagger_{13} + 4.6188c^\dagger_{0}c^\dagger_{1}c^\dagger_{3}c^\dagger_{5}c^\dagger_{8}c^\dagger_{9}c^\dagger_{11}c^\dagger_{13} + 5.0c^\dagger_{0}c^\dagger_{1}c^\dagger_{3}c^\dagger_{6}c^\dagger_{7}c^\dagger_{9}c^\dagger_{11}c^\dagger_{13} - 28.5689c^\dagger_{0}c^\dagger_{1}c^\dagger_{3}c^\dagger_{6}c^\dagger_{8}c^\dagger_{9}c^\dagger_{10}c^\dagger_{13} \\
&- 3.41565c^\dagger_{0}c^\dagger_{1}c^\dagger_{4}c^\dagger_{5}c^\dagger_{6}c^\dagger_{10}c^\dagger_{11}c^\dagger_{13} - 10.6145c^\dagger_{0}c^\dagger_{1}c^\dagger_{4}c^\dagger_{5}c^\dagger_{7}c^\dagger_{9}c^\dagger_{11}c^\dagger_{13} + 7.65942c^\dagger_{0}c^\dagger_{1}c^\dagger_{4}c^\dagger_{5}c^\dagger_{8}c^\dagger_{9}c^\dagger_{10}c^\dagger_{13} + 3.0c^\dagger_{0}c^\dagger_{1}c^\dagger_{4}c^\dagger_{6}c^\dagger_{7}c^\dagger_{8}c^\dagger_{11}c^\dagger_{13} \\
&+ 30.7542c^\dagger_{0}c^\dagger_{1}c^\dagger_{4}c^\dagger_{6}c^\dagger_{7}c^\dagger_{9}c^\dagger_{10}c^\dagger_{13} - 47.8682c^\dagger_{0}c^\dagger_{1}c^\dagger_{5}c^\dagger_{6}c^\dagger_{7}c^\dagger_{8}c^\dagger_{10}c^\dagger_{13} - 2.04124c^\dagger_{0}c^\dagger_{2}c^\dagger_{3}c^\dagger_{4}c^\dagger_{7}c^\dagger_{10}c^\dagger_{11}c^\dagger_{13} - 7.30297c^\dagger_{0}c^\dagger_{2}c^\dagger_{3}c^\dagger_{4}c^\dagger_{8}c^\dagger_{9}c^\dagger_{11}c^\dagger_{13} \\
&+ 2.41523c^\dagger_{0}c^\dagger_{2}c^\dagger_{3}c^\dagger_{5}c^\dagger_{6}c^\dagger_{10}c^\dagger_{11}c^\dagger_{13} - 2.3094c^\dagger_{0}c^\dagger_{2}c^\dagger_{3}c^\dagger_{5}c^\dagger_{7}c^\dagger_{9}c^\dagger_{11}c^\dagger_{13} + 27.8187c^\dagger_{0}c^\dagger_{2}c^\dagger_{3}c^\dagger_{5}c^\dagger_{8}c^\dagger_{9}c^\dagger_{10}c^\dagger_{13} - 10.6066c^\dagger_{0}c^\dagger_{2}c^\dagger_{3}c^\dagger_{6}c^\dagger_{7}c^\dagger_{8}c^\dagger_{11}c^\dagger_{13} \\
&+ 1.91881c^\dagger_{0}c^\dagger_{2}c^\dagger_{3}c^\dagger_{6}c^\dagger_{7}c^\dagger_{9}c^\dagger_{10}c^\dagger_{13} + 18.3303c^\dagger_{0}c^\dagger_{2}c^\dagger_{4}c^\dagger_{5}c^\dagger_{6}c^\dagger_{9}c^\dagger_{11}c^\dagger_{13} + 13.8564c^\dagger_{0}c^\dagger_{2}c^\dagger_{4}c^\dagger_{5}c^\dagger_{7}c^\dagger_{8}c^\dagger_{11}c^\dagger_{13} - 43.6935c^\dagger_{0}c^\dagger_{2}c^\dagger_{4}c^\dagger_{5}c^\dagger_{7}c^\dagger_{9}c^\dagger_{10}c^\dagger_{13} \\
&+ 3.41121c^\dagger_{0}c^\dagger_{2}c^\dagger_{4}c^\dagger_{6}c^\dagger_{7}c^\dagger_{8}c^\dagger_{10}c^\dagger_{13} + 107.037c^\dagger_{0}c^\dagger_{2}c^\dagger_{5}c^\dagger_{6}c^\dagger_{7}c^\dagger_{8}c^\dagger_{9}c^\dagger_{13} - 44.9778c^\dagger_{0}c^\dagger_{3}c^\dagger_{4}c^\dagger_{5}c^\dagger_{6}c^\dagger_{8}c^\dagger_{11}c^\dagger_{13} + 12.7636c^\dagger_{0}c^\dagger_{3}c^\dagger_{4}c^\dagger_{5}c^\dagger_{6}c^\dagger_{9}c^\dagger_{10}c^\dagger_{13} \\
&+ 62.1113c^\dagger_{0}c^\dagger_{3}c^\dagger_{4}c^\dagger_{5}c^\dagger_{7}c^\dagger_{8}c^\dagger_{10}c^\dagger_{13} - 123.781c^\dagger_{0}c^\dagger_{3}c^\dagger_{4}c^\dagger_{6}c^\dagger_{7}c^\dagger_{8}c^\dagger_{9}c^\dagger_{13} + 24.5289c^\dagger_{1}c^\dagger_{2}c^\dagger_{3}c^\dagger_{4}c^\dagger_{7}c^\dagger_{9}c^\dagger_{11}c^\dagger_{13} - 37.9832c^\dagger_{1}c^\dagger_{2}c^\dagger_{3}c^\dagger_{4}c^\dagger_{8}c^\dagger_{9}c^\dagger_{10}c^\dagger_{13} \\
&- 29.023c^\dagger_{1}c^\dagger_{2}c^\dagger_{3}c^\dagger_{5}c^\dagger_{6}c^\dagger_{9}c^\dagger_{11}c^\dagger_{13} - 8.66025c^\dagger_{1}c^\dagger_{2}c^\dagger_{3}c^\dagger_{5}c^\dagger_{7}c^\dagger_{8}c^\dagger_{11}c^\dagger_{13} + 11.6632c^\dagger_{1}c^\dagger_{2}c^\dagger_{3}c^\dagger_{5}c^\dagger_{7}c^\dagger_{9}c^\dagger_{10}c^\dagger_{13} + 22.5993c^\dagger_{1}c^\dagger_{2}c^\dagger_{3}c^\dagger_{6}c^\dagger_{7}c^\dagger_{8}c^\dagger_{10}c^\dagger_{13} \\
&+ 22.9129c^\dagger_{1}c^\dagger_{2}c^\dagger_{4}c^\dagger_{5}c^\dagger_{6}c^\dagger_{8}c^\dagger_{11}c^\dagger_{13} + 32.7002c^\dagger_{1}c^\dagger_{2}c^\dagger_{4}c^\dagger_{5}c^\dagger_{6}c^\dagger_{9}c^\dagger_{10}c^\dagger_{13} - 30.8117c^\dagger_{1}c^\dagger_{2}c^\dagger_{4}c^\dagger_{5}c^\dagger_{7}c^\dagger_{8}c^\dagger_{10}c^\dagger_{13} - 35.7326c^\dagger_{1}c^\dagger_{2}c^\dagger_{4}c^\dagger_{6}c^\dagger_{7}c^\dagger_{8}c^\dagger_{9}c^\dagger_{13} \\
&+ 14.9666c^\dagger_{1}c^\dagger_{3}c^\dagger_{4}c^\dagger_{5}c^\dagger_{6}c^\dagger_{7}c^\dagger_{11}c^\dagger_{13} - 53.4475c^\dagger_{1}c^\dagger_{3}c^\dagger_{4}c^\dagger_{5}c^\dagger_{6}c^\dagger_{8}c^\dagger_{10}c^\dagger_{13} + 106.788c^\dagger_{1}c^\dagger_{3}c^\dagger_{4}c^\dagger_{5}c^\dagger_{7}c^\dagger_{8}c^\dagger_{9}c^\dagger_{13} + 71.7952c^\dagger_{2}c^\dagger_{3}c^\dagger_{4}c^\dagger_{5}c^\dagger_{6}c^\dagger_{7}c^\dagger_{10}c^\dagger_{13} \\
&- 80.2694c^\dagger_{2}c^\dagger_{3}c^\dagger_{4}c^\dagger_{5}c^\dagger_{6}c^\dagger_{8}c^\dagger_{9}c^\dagger_{13} + 10.0256c^\dagger_{0}c^\dagger_{1}c^\dagger_{2}c^\dagger_{6}c^\dagger_{8}c^\dagger_{10}c^\dagger_{11}c^\dagger_{12} - 29.3581c^\dagger_{0}c^\dagger_{1}c^\dagger_{2}c^\dagger_{7}c^\dagger_{8}c^\dagger_{9}c^\dagger_{11}c^\dagger_{12} - 14.1784c^\dagger_{0}c^\dagger_{1}c^\dagger_{3}c^\dagger_{5}c^\dagger_{8}c^\dagger_{10}c^\dagger_{11}c^\dagger_{12} \\
&- 14.4715c^\dagger_{0}c^\dagger_{1}c^\dagger_{3}c^\dagger_{6}c^\dagger_{7}c^\dagger_{10}c^\dagger_{11}c^\dagger_{12} + 33.3397c^\dagger_{0}c^\dagger_{1}c^\dagger_{3}c^\dagger_{6}c^\dagger_{8}c^\dagger_{9}c^\dagger_{11}c^\dagger_{12} + 8.76101c^\dagger_{0}c^\dagger_{1}c^\dagger_{3}c^\dagger_{7}c^\dagger_{8}c^\dagger_{9}c^\dagger_{10}c^\dagger_{12} + 31.8671c^\dagger_{0}c^\dagger_{1}c^\dagger_{4}c^\dagger_{5}c^\dagger_{7}c^\dagger_{10}c^\dagger_{11}c^\dagger_{12} \\
&+ 0.640513c^\dagger_{0}c^\dagger_{1}c^\dagger_{4}c^\dagger_{5}c^\dagger_{8}c^\dagger_{9}c^\dagger_{11}c^\dagger_{12} - 44.0987c^\dagger_{0}c^\dagger_{1}c^\dagger_{4}c^\dagger_{6}c^\dagger_{7}c^\dagger_{9}c^\dagger_{11}c^\dagger_{12} - 17.9759c^\dagger_{0}c^\dagger_{1}c^\dagger_{4}c^\dagger_{6}c^\dagger_{8}c^\dagger_{9}c^\dagger_{10}c^\dagger_{12} + 65.7384c^\dagger_{0}c^\dagger_{1}c^\dagger_{5}c^\dagger_{6}c^\dagger_{7}c^\dagger_{8}c^\dagger_{11}c^\dagger_{12} \\
&+ 29.7313c^\dagger_{0}c^\dagger_{1}c^\dagger_{5}c^\dagger_{6}c^\dagger_{7}c^\dagger_{9}c^\dagger_{10}c^\dagger_{12} + 22.4179c^\dagger_{0}c^\dagger_{2}c^\dagger_{3}c^\dagger_{4}c^\dagger_{8}c^\dagger_{10}c^\dagger_{11}c^\dagger_{12} + 5.0637c^\dagger_{0}c^\dagger_{2}c^\dagger_{3}c^\dagger_{5}c^\dagger_{7}c^\dagger_{10}c^\dagger_{11}c^\dagger_{12} - 38.7239c^\dagger_{0}c^\dagger_{2}c^\dagger_{3}c^\dagger_{5}c^\dagger_{8}c^\dagger_{9}c^\dagger_{11}c^\dagger_{12} \\
&+ 15.2971c^\dagger_{0}c^\dagger_{2}c^\dagger_{3}c^\dagger_{6}c^\dagger_{7}c^\dagger_{9}c^\dagger_{11}c^\dagger_{12} + 3.67946c^\dagger_{0}c^\dagger_{2}c^\dagger_{3}c^\dagger_{6}c^\dagger_{8}c^\dagger_{9}c^\dagger_{10}c^\dagger_{12} - 50.9097c^\dagger_{0}c^\dagger_{2}c^\dagger_{4}c^\dagger_{5}c^\dagger_{6}c^\dagger_{10}c^\dagger_{11}c^\dagger_{12} + 30.9047c^\dagger_{0}c^\dagger_{2}c^\dagger_{4}c^\dagger_{5}c^\dagger_{7}c^\dagger_{9}c^\dagger_{11}c^\dagger_{12} \\
&+ 10.1053c^\dagger_{0}c^\dagger_{2}c^\dagger_{4}c^\dagger_{5}c^\dagger_{8}c^\dagger_{9}c^\dagger_{10}c^\dagger_{12} - 18.0427c^\dagger_{0}c^\dagger_{2}c^\dagger_{4}c^\dagger_{6}c^\dagger_{7}c^\dagger_{8}c^\dagger_{11}c^\dagger_{12} + 13.955c^\dagger_{0}c^\dagger_{2}c^\dagger_{4}c^\dagger_{6}c^\dagger_{7}c^\dagger_{9}c^\dagger_{10}c^\dagger_{12} - 95.1995c^\dagger_{0}c^\dagger_{2}c^\dagger_{5}c^\dagger_{6}c^\dagger_{7}c^\dagger_{8}c^\dagger_{10}c^\dagger_{12} \\
&+ 52.0998c^\dagger_{0}c^\dagger_{3}c^\dagger_{4}c^\dagger_{5}c^\dagger_{6}c^\dagger_{9}c^\dagger_{11}c^\dagger_{12} - 43.544c^\dagger_{0}c^\dagger_{3}c^\dagger_{4}c^\dagger_{5}c^\dagger_{7}c^\dagger_{8}c^\dagger_{11}c^\dagger_{12} - 58.6206c^\dagger_{0}c^\dagger_{3}c^\dagger_{4}c^\dagger_{5}c^\dagger_{7}c^\dagger_{9}c^\dagger_{10}c^\dagger_{12} + 93.8152c^\dagger_{0}c^\dagger_{3}c^\dagger_{4}c^\dagger_{6}c^\dagger_{7}c^\dagger_{8}c^\dagger_{10}c^\dagger_{12} \\
&+ 15.2083c^\dagger_{0}c^\dagger_{3}c^\dagger_{5}c^\dagger_{6}c^\dagger_{7}c^\dagger_{8}c^\dagger_{9}c^\dagger_{12} - 67.3705c^\dagger_{1}c^\dagger_{2}c^\dagger_{3}c^\dagger_{4}c^\dagger_{7}c^\dagger_{10}c^\dagger_{11}c^\dagger_{12} + 42.0287c^\dagger_{1}c^\dagger_{2}c^\dagger_{3}c^\dagger_{4}c^\dagger_{8}c^\dagger_{9}c^\dagger_{11}c^\dagger_{12} + 79.7138c^\dagger_{1}c^\dagger_{2}c^\dagger_{3}c^\dagger_{5}c^\dagger_{6}c^\dagger_{10}c^\dagger_{11}c^\dagger_{12} \\
&+ 2.56205c^\dagger_{1}c^\dagger_{2}c^\dagger_{3}c^\dagger_{5}c^\dagger_{7}c^\dagger_{9}c^\dagger_{11}c^\dagger_{12} - 1.09246c^\dagger_{1}c^\dagger_{2}c^\dagger_{3}c^\dagger_{5}c^\dagger_{8}c^\dagger_{9}c^\dagger_{10}c^\dagger_{12} + 28.4368c^\dagger_{1}c^\dagger_{2}c^\dagger_{3}c^\dagger_{6}c^\dagger_{7}c^\dagger_{8}c^\dagger_{11}c^\dagger_{12} - 95.97c^\dagger_{1}c^\dagger_{2}c^\dagger_{3}c^\dagger_{6}c^\dagger_{7}c^\dagger_{9}c^\dagger_{10}c^\dagger_{12} \\
&- 77.106c^\dagger_{1}c^\dagger_{2}c^\dagger_{4}c^\dagger_{5}c^\dagger_{6}c^\dagger_{9}c^\dagger_{11}c^\dagger_{12} - 23.0585c^\dagger_{1}c^\dagger_{2}c^\dagger_{4}c^\dagger_{5}c^\dagger_{7}c^\dagger_{8}c^\dagger_{11}c^\dagger_{12} + 93.8089c^\dagger_{1}c^\dagger_{2}c^\dagger_{4}c^\dagger_{5}c^\dagger_{7}c^\dagger_{9}c^\dagger_{10}c^\dagger_{12} + 56.0564c^\dagger_{1}c^\dagger_{2}c^\dagger_{4}c^\dagger_{6}c^\dagger_{7}c^\dagger_{8}c^\dagger_{10}c^\dagger_{12} \\
&- 111.22c^\dagger_{1}c^\dagger_{2}c^\dagger_{5}c^\dagger_{6}c^\dagger_{7}c^\dagger_{8}c^\dagger_{9}c^\dagger_{12} + 121.077c^\dagger_{1}c^\dagger_{3}c^\dagger_{4}c^\dagger_{5}c^\dagger_{6}c^\dagger_{8}c^\dagger_{11}c^\dagger_{12} - 63.7197c^\dagger_{1}c^\dagger_{3}c^\dagger_{4}c^\dagger_{5}c^\dagger_{6}c^\dagger_{9}c^\dagger_{10}c^\dagger_{12} - 133.464c^\dagger_{1}c^\dagger_{3}c^\dagger_{4}c^\dagger_{5}c^\dagger_{7}c^\dagger_{8}c^\dagger_{10}c^\dagger_{12} \\
&+ 115.623c^\dagger_{1}c^\dagger_{3}c^\dagger_{4}c^\dagger_{6}c^\dagger_{7}c^\dagger_{8}c^\dagger_{9}c^\dagger_{12} - 280.311c^\dagger_{2}c^\dagger_{3}c^\dagger_{4}c^\dagger_{5}c^\dagger_{6}c^\dagger_{7}c^\dagger_{11}c^\dagger_{12} + 237.173c^\dagger_{2}c^\dagger_{3}c^\dagger_{4}c^\dagger_{5}c^\dagger_{6}c^\dagger_{8}c^\dagger_{10}c^\dagger_{12} - 174.087c^\dagger_{2}c^\dagger_{3}c^\dagger_{4}c^\dagger_{5}c^\dagger_{7}c^\dagger_{8}c^\dagger_{9}c^\dagger_{12} \\
&+ 51.8462c^\dagger_{0}c^\dagger_{1}c^\dagger_{4}c^\dagger_{7}c^\dagger_{8}c^\dagger_{9}c^\dagger_{10}c^\dagger_{11} - 54.5054c^\dagger_{0}c^\dagger_{1}c^\dagger_{5}c^\dagger_{6}c^\dagger_{8}c^\dagger_{9}c^\dagger_{10}c^\dagger_{11} - 94.7817c^\dagger_{0}c^\dagger_{2}c^\dagger_{3}c^\dagger_{7}c^\dagger_{8}c^\dagger_{9}c^\dagger_{10}c^\dagger_{11} + 33.217c^\dagger_{0}c^\dagger_{2}c^\dagger_{4}c^\dagger_{6}c^\dagger_{8}c^\dagger_{9}c^\dagger_{10}c^\dagger_{11} \\
&+ 36.1843c^\dagger_{0}c^\dagger_{2}c^\dagger_{5}c^\dagger_{6}c^\dagger_{7}c^\dagger_{9}c^\dagger_{10}c^\dagger_{11} + 53.0527c^\dagger_{0}c^\dagger_{3}c^\dagger_{4}c^\dagger_{5}c^\dagger_{8}c^\dagger_{9}c^\dagger_{10}c^\dagger_{11} - 84.7351c^\dagger_{0}c^\dagger_{3}c^\dagger_{4}c^\dagger_{6}c^\dagger_{7}c^\dagger_{9}c^\dagger_{10}c^\dagger_{11} + 43.5009c^\dagger_{0}c^\dagger_{3}c^\dagger_{5}c^\dagger_{6}c^\dagger_{7}c^\dagger_{8}c^\dagger_{10}c^\dagger_{11} \\
&- 73.1712c^\dagger_{0}c^\dagger_{4}c^\dagger_{5}c^\dagger_{6}c^\dagger_{7}c^\dagger_{8}c^\dagger_{9}c^\dagger_{11} + 171.589c^\dagger_{1}c^\dagger_{2}c^\dagger_{3}c^\dagger_{6}c^\dagger_{8}c^\dagger_{9}c^\dagger_{10}c^\dagger_{11} - 208.26c^\dagger_{1}c^\dagger_{2}c^\dagger_{4}c^\dagger_{5}c^\dagger_{8}c^\dagger_{9}c^\dagger_{10}c^\dagger_{11} - 76.4382c^\dagger_{1}c^\dagger_{2}c^\dagger_{4}c^\dagger_{6}c^\dagger_{7}c^\dagger_{9}c^\dagger_{10}c^\dagger_{11} \\
&+ 145.882c^\dagger_{1}c^\dagger_{2}c^\dagger_{5}c^\dagger_{6}c^\dagger_{7}c^\dagger_{8}c^\dagger_{10}c^\dagger_{11} + 260.57c^\dagger_{1}c^\dagger_{3}c^\dagger_{4}c^\dagger_{5}c^\dagger_{7}c^\dagger_{9}c^\dagger_{10}c^\dagger_{11} - 168.051c^\dagger_{1}c^\dagger_{3}c^\dagger_{4}c^\dagger_{6}c^\dagger_{7}c^\dagger_{8}c^\dagger_{10}c^\dagger_{11} - 43.9027c^\dagger_{1}c^\dagger_{3}c^\dagger_{5}c^\dagger_{6}c^\dagger_{7}c^\dagger_{8}c^\dagger_{9}c^\dagger_{11} \\
&- 331.4c^\dagger_{2}c^\dagger_{3}c^\dagger_{4}c^\dagger_{5}c^\dagger_{6}c^\dagger_{9}c^\dagger_{10}c^\dagger_{11} + 65.2405c^\dagger_{2}c^\dagger_{3}c^\dagger_{4}c^\dagger_{5}c^\dagger_{7}c^\dagger_{8}c^\dagger_{10}c^\dagger_{11} + 161.971c^\dagger_{2}c^\dagger_{3}c^\dagger_{4}c^\dagger_{6}c^\dagger_{7}c^\dagger_{8}c^\dagger_{9}c^\dagger_{11} + 242.681c^\dagger_{1}c^\dagger_{4}c^\dagger_{5}c^\dagger_{6}c^\dagger_{7}c^\dagger_{8}c^\dagger_{9}c^\dagger_{10} \\
&- 240.242c^\dagger_{2}c^\dagger_{3}c^\dagger_{5}c^\dagger_{6}c^\dagger_{7}c^\dagger_{8}c^\dagger_{9}c^\dagger_{10}\big)\, |0\rangle\,.
\end{aligned}
\tag{1.4}
$$
